# Supplementary material for: Unbiased Parameter Estimation via DREM with Annihilators
Source: arXiv:2403.11076 ancillary file (2024-12-11)
Supplement: Supplementary file 1 [file supp.pdf]

# Supplement to "Unbiased Parameter Estimation via DREM with Annihilators"

Anton Glushchenko, *Member, IEEE* and Konstantin Lastochkin

**Abstract**

This article is a supplementary material for "Unbiased Parameter Estimation via DREM with Annihilators" by the same authors. It presents proof of Theorem 2.

## Proof of Theorem 2

The regressor $\omega(t)$ is defined as:

$$\begin{array}{l}\omega(t) = \det\left\{\frac{k}{s+k}\left[\det\{\mathcal{H}^\top \text{adj}\{\Phi(t)\}\mathcal{L}_1\}\Phi(t)\right]\right\},\\ \Phi(t) = \frac{1}{T}\int\limits_{\max\{t_0,\, t-T\}}^{t} \phi(s)\phi^\top(s)\,ds,\end{array} \tag{A1}$$

Then, as **C1** and **C3** are met, for all $t \geq T_f$ we have

$$\begin{array}{l}\overline{\alpha} I_{2n} \geq \Phi(t) \geq \underline{\alpha} I_{2n} > 0,\\ \overline{\beta} \geq \left|\det\left\{\mathcal{H}^\top \text{adj}\{\Phi(t)\}\mathcal{L}_1\right\}\right| \geq \underline{\beta} > 0\end{array} \tag{A2}$$

and, consequently, there exists $\overline{T}_f \geq T_f$ such that

$$\left(\overline{\alpha}\overline{\beta}\right)^{2n} \geq |\omega(t)| \geq \left(\underline{\alpha}\underline{\beta}\right)^{2n} > 0,\, \forall t \geq \overline{T}_f. \tag{A3}$$

So, taking into consideration (A3), the following error is well defined for all $t \geq \overline{T}_f$:

$$\tilde{\kappa}(t) = \hat{\kappa}(t) - \omega^{-1}(t),$$

which is differentiated with respect to time and owing to

$$\begin{array}{c}\omega(t)\omega^{-1}(t) = 1 \Leftrightarrow \dot{\omega}(t)\omega^{-1}(t) + \omega(t)\frac{d\omega^{-1}(t)}{dt} = 0\\ \Updownarrow\\ \frac{d\omega^{-1}(t)}{dt} = -\dot{\omega}(t)\omega^{-2}(t),\end{array}$$

it is obtained:

$$\begin{array}{l}\dot{\tilde{\kappa}} = -\gamma\omega(\omega\hat{\kappa} - 1) - \dot{\omega}\hat{\kappa}^2 + \dot{\omega}\omega^{-2} =\\ = -\gamma\omega^2\tilde{\kappa} - \dot{\omega}\left(\hat{\kappa} + \omega^{-1}\right)\tilde{\kappa} =\\ = -\left(\gamma\omega^2 + \dot{\omega}\hat{\kappa} + \dot{\omega}\omega^{-1}\right)\tilde{\kappa}.\end{array} \tag{A4}$$

The quadratic form $V(t) = \frac{1}{2}\tilde{\kappa}^2(t)$ is introduced, which derivative is written as:

$$\dot{V}(t) = -2\left(\gamma\omega^2(t) + \dot{\omega}(t)\hat{\kappa}(t) + \dot{\omega}(t)\omega^{-1}(t)\right)V(t),$$

from which, when $\gamma\omega^3(t) + \omega(t)\dot{\omega}(t)\hat{\kappa}(t) + \dot{\omega}(t) \geq \eta\omega(t) > 0\ \forall t \geq \overline{T}_f$, then for all $t \geq \overline{T}_f$ there exists the following upper bound:

$$|\tilde{\kappa}(t)| \leq e^{-\eta\left(t - \overline{T}_f\right)}|\tilde{\kappa}(t_0)|. \tag{A5}$$

For all $t \geq \overline{T}_f$ $\hat{\theta}(t)$ is rewritten in the following form:

$$\begin{array}{l}\hat{\theta}(t) = \hat{\kappa}(t)\mathcal{L}_0\Lambda(t) \pm \omega^{-1}(t)\mathcal{L}_0\Lambda(t) =\\ = \omega^{-1}(t)\mathcal{L}_0\Lambda(t) + \tilde{\kappa}(t)\mathcal{L}_0\Lambda(t) =\\ = \theta + \omega^{-1}(t)\mathcal{L}_0\text{adj}\{\Omega_f(t)\}\frac{k}{s+k}\left[\left[\mathcal{M}(t)\mathcal{L}_2 - \right.\right.\\ \quad \left. -\mathcal{L}_1\text{adj}\{\mathcal{H}^\top \text{adj}\{\Phi(t)\}\mathcal{L}_1\}\mathcal{H}^\top \text{adj}\{\Phi(t)\}\mathcal{L}_2\right] \times\\ \left. \times\mathcal{L}_2^\top W(t)\right] + \tilde{\kappa}(t)\mathcal{L}_0\Lambda(t).\end{array} \tag{A6}$$

When **C1** and **C3** are met, then, according to (A2), for all $t \geq \overline{T}_f$ it holds that:

$$0 < \left|\omega^{-1}(t)\right| \leq \left(\underline{\alpha}\underline{\beta}\right)^{-2n},\ \text{adj}\{\Omega_f\} \leq \left(\overline{\alpha}\overline{\beta}\right)^{2n-1} I_{2n},$$

A. Glushchenko is with V.A. Trapeznikov Institute of Control Sciences of Russian Academy of Sciences, Moscow, Russia aiglush@ipu.ru
K. Lastochkin is with V.A. Trapeznikov Institute of Control Sciences of Russian Academy of Sciences, Moscow, Russia lastconst@ipu.ru

and consequently, from (A6) we have the following upper bound of the error $\tilde{\theta}(t)$:

$$\begin{gathered}\left\|\tilde{\theta}(t)\right\| \leqslant \left(\underline{\alpha}\underline{\beta}\right)^{-2n}\left(\overline{\alpha}\overline{\beta}\right)^{2n-1}\left\|\tfrac{k}{s+k}\left[\left[\mathcal{M}(t)\mathcal{L}_2 - \right.\right.\right.\\ \left. -\mathcal{L}_1\text{adj}\{\mathcal{H}^\top\text{adj}\{\Phi(t)\}\mathcal{L}_1\}\mathcal{H}^\top\text{adj}\{\Phi(t)\}\mathcal{L}_2\right]\times \\ \left.\left.\times\mathcal{L}_2^\top W(t)\right]\right\| + e^{-\eta\left(t-\overline{T}_f\right)}\left|\tilde{\kappa}(t_0)\right|\left\|\Lambda(t)\right\|.\end{gathered} \quad \text{(A7)}$$

When **C2** is met, then, following (11), it holds that:

$$\lim_{T\to\infty}\mathcal{L}_2^\top W(t) = \lim_{T\to\infty}\tfrac{1}{T}\mathcal{L}_2^\top\int\limits_{\max\{t_0,\, t-T\}}^{t}\phi(s)f(s)\,ds = 0$$

from which, as $\Lambda(t)$ and

$$\mathcal{M}(t)\mathcal{L}_2 - \mathcal{L}_1\text{adj}\left\{\mathcal{H}^\top\text{adj}\{\Phi(t)\}\mathcal{L}_1\right\}\mathcal{H}^\top\text{adj}\{\Phi(t)\}\mathcal{L}_2$$

are bounded, for bounded $\varphi(t)$, $w(t)$ and any $T>0$ there exists $c>0$ such that:

$$\begin{gathered}\lim_{t\to\infty}\left\|\tilde{\theta}(t)\right\| \leqslant \left(\underline{\alpha}\underline{\beta}\right)^{-2n}\left(\overline{\alpha}\overline{\beta}\right)^{2n-1}\left\|\tfrac{k}{s+k}\left[\left[\mathcal{M}(t)\mathcal{L}_2 - \right.\right.\right.\\ \left.\left.\left. -\mathcal{L}_1\text{adj}\{\mathcal{H}^\top\text{adj}\{\Phi(t)\}\mathcal{L}_1\}\mathcal{H}^\top\text{adj}\{\Phi(t)\}\mathcal{L}_2\right]\mathcal{L}_2^\top W(t)\right]\right\| \\ \leqslant c\left\|\lim_{t\to\infty}\tfrac{k}{s+k}\left\{\mathcal{L}_2^\top W(t)\right\}\right\| := \varepsilon(T), \\ \lim_{T\to\infty}\varepsilon(T) = c\left\|\lim_{t\to\infty}\lim_{T\to\infty}\tfrac{k}{s+k}\left\{\mathcal{L}_2^\top W(t)\right\}\right\| = \\ = c\left\|\lim_{t\to\infty}\tfrac{k}{s+k}\left\{\lim_{T\to\infty}\mathcal{L}_2^\top W(t)\right\}\right\| = 0,\end{gathered}$$

which was to be proved.
